# Supplementary material for: High-Level Coupled-Cluster Energetics by Monte Carlo Sampling and Moment Expansions: Further Details and Comparisons
Source: arXiv:2102.10158 ancillary file (2021-03-17)
Supplement: Supplementary file 1 [file supplementary-material.pdf]

# High-Level Coupled-Cluster Energetics by Monte Carlo Sampling and Moment Expansions: Further Details and Comparisons (Supplementary Material)

J. Emiliano Deustua,[1] Jun Shen,[1] and Piotr Piecuch[1, 2, a)]

[1)] *Department of Chemistry, Michigan State University, East Lansing, Michigan 48824, USA*

[2)] *Department of Physics and Astronomy, Michigan State University, East Lansing, Michigan 48824, USA*

This document provides the information about the total numbers of walkers characterizing the various CIQMC propagations carried out in this study. The total numbers of walkers used in the FCIQMC, CISDT-MC, and CISDTQ-MC propagations that were needed to generate the CC($P$) and CC($P$;$Q$) results for the fluorine molecule, as described by the cc-pVDZ basis set, in which the internuclear separation $R$ was set at $R_e$, $1.5R_e$, $2R_e$, and $5R_e$, reported in Table I of the main text, can be found in Table S.1. The total numbers of walkers characterizing the FCIQMC, CISDT-MC, and CISDTQ-MC propagations that were used to obtain the CC($P$) and CC($P$;$Q$) energies for the stretched $F_2$ system, in which the F–F distance $R$ was set at $2R_e$ and the cc-pVTZ and aug-cc-pVTZ basis sets were employed, presented in Table II of the main text, are shown in Table S.2. The total numbers of walkers used in the FCIQMC, CISDT-MC, and CISDTQ-MC propagations for the reactant and transition-state structures defining the automerization of cyclobutadiene, as described by the cc-pVDZ basis set, which were needed to determine the CC($P$) and CC($P$;$Q$) data reported in Table III of the main text, can be found in Table S.3. Finally, Table S.4 shows the total numbers of walkers characterizing the FCIQMC and CISDTQ-MC propagations for the water molecule, as described by the cc-pVDZ basis set, at the equilibrium and four displaced geometries that represent a simultaneous stretching of both O–H bonds by factors of 1.5, 2.0, 2.5, and 3.0 without changing the ∠(H–O–H) angle, which were used to generate the CC($P$) and CC($P$;$Q$) energies presented in Table IV of the main text.

[a)] Corresponding author; e-mail: piecuch@chemistry.msu.edu.

TABLE S.1. The total numbers of walkers, reported as percentages of the total walker populations at 120,000 MC iterations, characterizing the $i$-FCIQMC, $i$-CISDTQ-MC, and $i$-CISDT-MC propagations with $\delta\tau = 0.0001$ a.u. that were needed to generate the CC($P$) and CC($P$;$Q$) results for the $F_2$ molecule reported in Table I of the main text. As in Table I, the cc-pVDZ basis set was employed and, in addition to the equilibrium geometry $R_e = 2.66816$ bohr, three stretches of the F–F bond, including $1.5R_e$, $2R_e$, and $5R_e$, were considered. The $i$-FCIQMC, $i$-CISDTQ-MC, and $i$-CISDT-MC calculations preceding the CC($P$) and CC($P$;$Q$) steps were initiated by placing 100 walkers on the RHF determinant and the $n_a$ parameter of the initiator algorithm was set at 3. The lowest two core orbitals were kept frozen and the Cartesian components of $d$ orbitals were employed throughout.

| $R/R_e$ | MC iterations | $i$-FCIQMC | $i$-CISDTQ-MC | $i$-CISDT-MC |
|---|---|---|---|---|
| 1.0 | 0 | 0.01[a] | 0.01[a] | 0.05[a] |
| | 10000 | 0.22 | 0.32 | 1.06 |
| | 20000 | 0.53 | 0.72 | 1.78 |
| | 30000 | 0.97 | 1.42 | 2.92 |
| | 40000 | 1.76 | 2.54 | 4.66 |
| | 50000 | 3.08 | 4.50 | 7.88 |
| | 60000 | 5.42 | 7.45 | 11.86 |
| | 70000 | 8.97 | 12.03 | 17.60 |
| | 80000 | 14.39 | 18.93 | 25.19 |
| | 100000 | 37.89 | 43.98 | 51.24 |
| | 120000 | 100[b] | 100[b] | 100[b] |
| 1.5 | 0 | 0.00[a] | 0.00[a] | 0.03[a] |
| | 10000 | 0.06 | 0.11 | 0.47 |
| | 20000 | 0.14 | 0.27 | 0.89 |
| | 30000 | 0.28 | 0.61 | 1.52 |
| | 40000 | 0.56 | 1.23 | 2.75 |
| | 50000 | 1.20 | 2.39 | 4.61 |
| | 60000 | 2.39 | 4.33 | 7.63 |
| | 70000 | 4.59 | 7.52 | 11.92 |
| | 80000 | 8.27 | 12.81 | 18.37 |
| | 100000 | 27.91 | 36.19 | 43.06 |
| | 120000 | 100[c] | 100[c] | 100[c] |
| 2.0 | 0 | 0.00[a] | 0.00[a] | 0.01[a] |
| | 10000 | 0.02 | 0.06 | 0.24 |
| | 20000 | 0.05 | 0.14 | 0.49 |
| | 30000 | 0.11 | 0.31 | 0.90 |
| | 40000 | 0.26 | 0.67 | 1.60 |
| | 50000 | 0.57 | 1.40 | 2.87 |
| | 60000 | 1.20 | 2.72 | 5.07 |
| | 70000 | 2.47 | 4.94 | 8.60 |
| | 80000 | 5.12 | 9.08 | 14.03 |
| | 100000 | 22.82 | 30.23 | 36.90 |
| | 120000 | 100[d] | 100[d] | 100[d] |
| 5.0 | 0 | 0.00[a] | 0.00[a] | 0.01[a] |
| | 10000 | 0.01 | 0.03 | 0.10 |
| | 20000 | 0.02 | 0.07 | 0.21 |
| | 30000 | 0.05 | 0.15 | 0.43 |
| | 40000 | 0.13 | 0.35 | 0.88 |
| | 50000 | 0.32 | 0.75 | 1.69 |
| | 60000 | 0.71 | 1.59 | 3.08 |
| | 70000 | 1.59 | 3.14 | 5.38 |
| | 80000 | 3.75 | 6.30 | 9.64 |
| | 100000 | 20.84 | 25.02 | 30.34 |
| | 120000 | 100[e] | 100[e] | 100[e] |

[a] The initial walker population, meaning 100 walkers on the RHF reference determinant.

[b] The total numbers of walkers at 120,000 MC iterations are 1,178,386 for $i$-FCIQMC, 805,751 for $i$-CISDTQ-MC, and 203,503 for $i$-CISDT-MC.

[c] The total numbers of walkers at 120,000 MC iterations are 4,770,245 for $i$-FCIQMC, 2,347,166 for $i$-CISDTQ-MC, and 391,574 for $i$-CISDT-MC.

[d] The total numbers of walkers at 120,000 MC iterations are 20,155,908 for $i$-FCIQMC, 5,419,152 for $i$-CISDTQ-MC, and 873,870 for $i$-CISDT-MC.

[e] The total numbers of walkers at 120,000 MC iterations are 41,817,674 for $i$-FCIQMC, 10,690,724 for $i$-CISDTQ-MC, and 1,929,384 for $i$-CISDT-MC.

TABLE S.2. The total numbers of walkers, reported as percentages of the total walker populations at 100,000 MC iterations, characterizing the $i$-FCIQMC, $i$-CISDTQ-MC, and $i$-CISDT-MC propagations with $\delta\tau = 0.0001$ a.u. that were needed to generate the CC($P$) and CC($P$;$Q$) results for the stretched $F_2$ molecule reported in Table II of the main text. As in Table II, the internuclear distance was set at twice the equilibrium bond length and the cc-pVTZ and aug-cc-pVTZ basis sets were employed. The $i$-FCIQMC, $i$-CISDTQ-MC, and $i$-CISDT-MC calculations preceding the CC($P$) and CC($P$;$Q$) steps were initiated by placing 100 walkers on the RHF determinant and the $n_a$ parameter of the initiator algorithm was set at 3. The lowest two core orbitals were kept frozen and the spherical components of $d$ and $f$ orbitals were employed throughout.

| Basis set | MC iterations | $i$-FCIQMC | $i$-CISDTQ-MC | $i$-CISDT-MC |
|---|---|---|---|---|
| cc-pVTZ | 0 | 0.00[a] | 0.00[a] | 0.00[a] |
| | 10000 | 0.01 | 0.03 | 0.22 |
| | 20000 | 0.03 | 0.10 | 0.49 |
| | 30000 | 0.10 | 0.31 | 1.09 |
| | 40000 | 0.30 | 0.86 | 2.48 |
| | 50000 | 0.83 | 2.16 | 5.04 |
| | 60000 | 2.12 | 5.01 | 9.83 |
| | 70000 | 5.34 | 10.89 | 18.24 |
| | 80000 | 13.95 | 22.95 | 32.35 |
| | 100000 | 100[b] | 100[b] | 100[b] |
| aug-cc-pVTZ | 0 | 0.00[a] | 0.00[a] | 0.00[a] |
| | 10000 | 0.00 | 0.02 | 0.12 |
| | 20000 | 0.02 | 0.07 | 0.35 |
| | 30000 | 0.06 | 0.22 | 0.81 |
| | 40000 | 0.19 | 0.62 | 1.87 |
| | 50000 | 0.60 | 1.66 | 4.31 |
| | 60000 | 1.69 | 4.17 | 9.09 |
| | 70000 | 4.54 | 9.60 | 17.61 |
| | 80000 | 12.21 | 21.31 | 32.71 |
| | 100000 | 100[c] | 100[c] | 100[c] |

[a] The initial walker population, meaning 100 walkers on the RHF reference determinant.

[b] The total numbers of walkers at 100,000 MC iterations are 77,776,442 for $i$-FCIQMC, 18,767,613 for $i$-CISDTQ-MC, and 2,072,885 for $i$-CISDT-MC.

[c] The total numbers of walkers at 100,000 MC iterations are 332,951,806 for $i$-FCIQMC, 68,536,538 for $i$-CISDTQ-MC, and 6,214,125 for $i$-CISDT-MC.

TABLE S.3. The total numbers of walkers, reported as percentages of the total walker populations at 80,000 MC iterations, characterizing the $i$-FCIQMC, $i$-CISDTQ-MC, and $i$-CISDT-MC propagations with $\delta\tau = 0.0001$ a.u. that were needed to generate the CC($P$) and CC($P$;$Q$) results for the reactant (R) and transition-state (TS) structures defining the automerization of cyclobutadiene reported in Table III of the main text. As in Table III, the cc-pVDZ basis set using the spherical components of $d$ orbitals was employed throughout and the lowest four core orbitals were kept frozen. The $i$-FCIQMC, $i$-CISDTQ-MC, and $i$-CISDT-MC calculations preceding the CC($P$) and CC($P$;$Q$) steps were initiated by placing 100 walkers on the RHF determinant and the $n_a$ parameter of the initiator algorithm was set at 3.

| Species | MC iterations | $i$-FCIQMC | $i$-CISDTQ-MC | $i$-CISDT-MC |
|---|---|---|---|---|
| R | 0 | 0.00[a] | 0.00[a] | 0.00[a] |
| | 10000 | 0.04 | 0.08 | 0.43 |
| | 20000 | 0.18 | 0.34 | 1.12 |
| | 30000 | 0.66 | 1.09 | 2.82 |
| | 40000 | 1.95 | 3.47 | 6.99 |
| | 50000 | 5.33 | 8.97 | 15.18 |
| | 60000 | 14.38 | 21.66 | 31.07 |
| | 70000 | 38.41 | 47.70 | 58.57 |
| | 80000 | 100[b] | 100[b] | 100[b] |
| TS | 0 | 0.00[a] | 0.00[a] | 0.00[a] |
| | 10000 | 0.05 | 0.08 | 0.39 |
| | 20000 | 0.16 | 0.37 | 0.98 |
| | 30000 | 0.60 | 1.08 | 2.82 |
| | 40000 | 1.87 | 3.15 | 7.29 |
| | 50000 | 5.39 | 8.42 | 16.46 |
| | 60000 | 14.63 | 20.88 | 32.75 |
| | 70000 | 37.46 | 47.38 | 59.58 |
| | 80000 | 100[c] | 100[c] | 100[c] |

[a] The initial walker population, meaning 100 walkers on the RHF reference determinant.

[b] The total numbers of walkers at 80,000 MC iterations are 42,892,242 for $i$-FCIQMC, 22,344,003 for $i$-CISDTQ-MC, and 2,845,325 for $i$-CISDT-MC.

[c] The total numbers of walkers at 80,000 MC iterations are 42,964,652 for $i$-FCIQMC, 21,045,047 for $i$-CISDTQ-MC, and 2,877,382 for $i$-CISDT-MC.

TABLE S.4. The total numbers of walkers, reported as percentages of the total walker populations at 100,000 MC iterations, characterizing the $i$-FCIQMC and $i$-CISDTQ-MC propagations with $\delta\tau = 0.0001$ a.u. that were needed to generate the CC($P$) and CC($P$;$Q$) results for the water molecule reported in Table IV of the main text. As in Table IV, the cc-pVDZ basis set was employed and, in addition to the equilibrium geometry $R_{\text{O-H}} = R_e$, four displaced geometries that represent a simultaneous stretching of both O–H bonds by factors of 1.5, 2.0, 2.5, and 3.0 without changing the ∠(H–O–H) angle were considered. The $i$-FCIQMC and $i$-CISDTQ-MC calculations preceding the CC($P$) and CC($P$;$Q$) steps were initiated by placing 100 walkers on the RHF determinant and the $n_a$ parameter of the initiator algorithm was set at 3. All electrons were correlated and the spherical components of $d$ orbitals were employed throughout.

| $R_{\text{O-H}}/R_e$ | MC iterations | $i$-FCIQMC | $i$-CISDTQ-MC |
|---|---|---|---|
| 1.0 | 0 | 0.39[a] | 0.42[a] |
| | 10000 | 5.63 | 5.99 |
| | 20000 | 8.11 | 9.03 |
| | 30000 | 12.17 | 10.41 |
| | 40000 | 18.10 | 17.89 |
| | 50000 | 22.02 | 25.82 |
| | 60000 | 32.18 | 34.64 |
| | 70000 | 44.14 | 45.77 |
| | 80000 | 54.26 | 60.64 |
| | 100000 | 100[b] | 100[b] |
| 1.5 | 0 | 0.17[a] | 0.17[a] |
| | 10000 | 2.97 | 3.07 |
| | 20000 | 5.54 | 5.89 |
| | 30000 | 9.44 | 9.17 |
| | 40000 | 15.01 | 14.15 |
| | 50000 | 22.24 | 20.58 |
| | 60000 | 30.63 | 30.18 |
| | 70000 | 41.22 | 41.94 |
| | 80000 | 54.90 | 55.13 |
| | 100000 | 100[c] | 100[c] |
| 2.0 | 0 | 0.09[a] | 0.12[a] |
| | 10000 | 1.26 | 1.83 |
| | 20000 | 2.78 | 3.74 |
| | 30000 | 4.92 | 5.94 |
| | 40000 | 7.62 | 9.63 |
| | 50000 | 12.82 | 16.19 |
| | 60000 | 19.33 | 23.79 |
| | 70000 | 30.65 | 35.24 |
| | 80000 | 44.81 | 50.01 |
| | 100000 | 100[d] | 100[d] |
| 2.5 | 0 | 0.03[a] | 0.07[a] |
| | 10000 | 0.49 | 1.07 |
| | 20000 | 1.14 | 2.23 |
| | 30000 | 2.38 | 3.66 |
| | 40000 | 4.35 | 6.48 |
| | 50000 | 7.83 | 10.51 |
| | 60000 | 13.45 | 16.49 |
| | 70000 | 23.10 | 27.11 |
| | 80000 | 38.92 | 42.38 |
| | 100000 | 100[e] | 100[e] |
| 3.0 | 0 | 0.02[a] | 0.04[a] |
| | 10000 | 0.35 | 0.74 |
| | 20000 | 0.79 | 1.46 |
| | 30000 | 1.51 | 2.36 |
| | 40000 | 3.01 | 4.24 |
| | 50000 | 5.43 | 7.96 |
| | 60000 | 10.22 | 13.20 |
| | 70000 | 18.27 | 22.05 |
| | 80000 | 32.64 | 36.76 |
| | 100000 | 100[f] | 100[f] |

[a] The initial walker population, meaning 100 walkers on the RHF reference determinant.
[b] The total numbers of walkers at 100,000 MC iterations are 25,359 for $i$-FCIQMC and 23,850 for $i$-CISDTQ-MC.
[c] The total numbers of walkers at 100,000 MC iterations are 59,445 for $i$-FCIQMC and 58,398 for $i$-CISDTQ-MC.
[d] The total numbers of walkers at 100,000 MC iterations are 115,212 for $i$-FCIQMC and 82,032 for $i$-CISDTQ-MC.
[e] The total numbers of walkers at 100,000 MC iterations are 320,443 for $i$-FCIQMC and 144,036 for $i$-CISDTQ-MC.
[f] The total numbers of walkers at 100,000 MC iterations are 454,916 for $i$-FCIQMC and 227,782 for $i$-CISDTQ-MC.
